# Supplementary material for: AKE-GNN: Effective Graph Learning with Adaptive Knowledge Exchange
Source: arXiv:2106.05455 source file (2023-10-04)
Supplement: Supplementary file 1 [file AppendixA-algorithm.tex]

\section{Pseudocode}
\label{sec:appendix-algorithm}
The pseudo-code of the AKE-GNN with the multiple GNNs is outlined in Algorithm~\ref{alg:gsl_4}. The training process involves generating multiple graph views, the individual learning phase, and the knowledge exchange phase. At the beginning~(Line 1-2), we generate multiple graph views via the graph augmentations. Then, in the individual learning phase~(Line 4-6), we train GNNs with the default hyperparameter settings and update the parameters of GNNs. At last, in the knowledge exchange phase~(Line 8-13), we utilize the entropy criterion to decide what is valuable information to exchange and propose an adaptive exchange strategy to substitute redundant output channels of one GNN~(target network) with informative channels of another GNN~(source network). Finally, we re-train the first network and obtain the final prediction~(Line 14).
\begin{algorithm}[]
    \caption{AKE-GNN with the multiple GNNs}
    \label{alg:gsl_4}
    \KwIn{The original graph $\gG$; number of multiple graph views $K$, $\gG_k$ denotes the $k$-th generated graph view; GNN~$\mathcal{F}_k$, whose input is $\gG_k$; $\bm{\theta}_{\gG_k}^l = \left[ \bm{\theta}_{\gG_k}^{l,1},\cdots,\bm{\theta}_{\gG_k}^{l,C_{l+1}} \right] \in \sR^{C_l \times C_{\left(l+1\right)}}$ denotes the weight in the $l$-th layer of a GNN corresponding to the $k$-th generated graph view, whose input channel is $C_l$ and output channel is $C_{\left(l+1\right)}$; the number layers of $\mathcal{F}_k$ is $L$; learning rate $\eta$; iteration steps $N$$\left(N >> K\right)$; number of exchange channels $M$; the graph augmentation functions $\mathcal{C}$ to get multiple graph views.}
  	\KwOut{Prediction $\mathbf{Z}$}
  	\For{$k = 1:K$}{
  	    Get the graph view $\mathcal{G}_k$ via the graph augmentation function $\mathcal{G}_k = \mathcal{C} \left(\mathcal{G}\right)$.\\
  	}
  	$\vartriangleright$ \textbf{The individual learning phase: } \\
  	\For{$k = 1:K$}{
  	    Train GNN~$\mathcal{F}_k\left(\mathcal{G}_k;\bm{\theta}_{\gG_k}\right)$ and compute the supervised classification loss $\mathcal{L}$.\\
  	    Update the weight $\bm{\theta}_{\gG_k}$ by gradient descent: $\bm{\theta}_{\gG_k} = \bm{\theta}_{\gG_k} - \eta \nabla_{\bm{\theta}}\mathcal{L}$. \\
  	}
  	$\vartriangleright$ \textbf{The knowledge exchange phase: } \\
  	\For{$n = \{1,\dots,N\}$}{
  	    Get the source and target GNN: $s = (n-1)\%K+1$, $t=n\%K+1$. \\
  	    \For{$l = \{1,\dots,L\}$, $m = \{1,\dots,M\}   \; \textbf{parallel}$}{
          	 Calculate the Pearson correlations among all possible pairs of the channels in $\bm{\theta}_{\gG_t}^l$. \\
      	    Find a pair of channels indexed by $\text{idx}_1$ and $\text{idx}_2$ with the highest correlation. \\
      	    Calculate and obtain the informative channel $i$ of the source network and the redundant channel $r$ of the target network as Eq.~\ref{eq:informative} and then exchange parameters between these two output channels. \\
  	    }
    }
    \textbf{Output} prediction $\mathbf{Z}$ via re-training $\mathbf{Z} = \mathcal{F}_1\left(\mathcal{G};\bm{\theta}_{\gG_1}\right)$. \\
    \tcc{\textbf{N.B.,} we use the first GNN by default as introduced in Sec.~\ref{sec:experiment-setup}.}
\end{algorithm}
