# Supplementary material for: AKE-GNN: Effective Graph Learning with Adaptive Knowledge Exchange
Source: arXiv:2106.05455 source file (2023-10-04)
Supplement: Supplementary file 2 [file AppendixD-datasets.tex]

\section{Datasets}
\label{sec:appendix-datasets}
\begin{table*}[]
\small
\caption{Statistics of the real-world datasets.}
\label{table:grpah-statistics}
\centering
\scalebox{1.}{
\setlength{\tabcolsep}{9pt} % Default value: 6pt
\begin{tabular}{lcccc}
\toprule
                                        & \textbf{\# Nodes:   $|\mathcal{V}|$} & \textbf{\# Edges:   $|\mathcal{E}|$}                      & \textbf{\# Features: d}                                   & \textbf{\# classes:   $|\mathcal{Y}|$} \\ \midrule[0.6pt]
\textbf{Cora}          & 2,708                                                 & 5,278                                                                      & 1,433                                                                      & 7                                                       \\
\textbf{CiteSeer}      & 3,327                                                 & 4,676                                                                      & 3,703                                                                      & 6                                                       \\
\textbf{PubMed}        & 19,717                                                & 44,327                                                                     & 500                                                                        & 3                                                       \\
\textbf{Chameleon}     & 2,277                                                 & 31,421                                                                     & 2,325                                                                      & 5                                                       \\
\textbf{Squirrel}      & 5,201                                                 & 198,493                                                                    & 2,089                                                                      & 5                                                       \\
\textbf{Actor}         & 7,600                                                 & 26,752                                                                     & 931                                                                        & 5                                                       \\
\textbf{Cornell}       & 183                                                   & 280                                                                        & 1,703                                                                      & 5                                                       \\
\textbf{Texas}         & 183                                                   & 295                                                                        & 1,703                                                                      & 5                                                       \\
\textbf{Wisconsin}     & 251                                                   & 466                                                                        & 1,703                                                                      & 5                                                       \\ \midrule
\textbf{OGBn-Arxiv}    & 169,343                                               & 1,166,243                                                                  & 128                                                                        & 40                                                      \\ \midrule\midrule
                                        & \textbf{\# Graphs: $|\mathcal{G}|$}  & \textbf{\tabincell{l}{\# Average nodes: \\ $|\mathcal{V}| / |\mathbb{G}|$}} & \textbf{\tabincell{l}{\# Average edges: \\ $|\mathcal{E}| / |\mathbb{G}|$}} & \textbf{\# classes: $|\mathcal{L}|$}   \\ \midrule[0.6pt]
\textbf{DD}            & 1,178                                                 & 284.32                                                                     & 715.66                                                                     & 2                                                       \\
\textbf{NCI1}          & 4,110                                                 & 29.87                                                                      & 32.30                                                                      & 2                                                       \\
\textbf{PROTEINS}      & 1,113                                                 & 39.06                                                                      & 72.82                                                                      & 2                                                       \\
\textbf{IMDB-BINARY}   & 1,000                                                 & 19.77                                                                      & 96.52                                                                      & 2                                                       \\
\textbf{REDDIT-BINARY} & 2,000                                                 & 429.63                                                                     & 497.75                                                                     & 2                                                       \\ \bottomrule
\end{tabular}
}
\end{table*}
In this section, we describe the details~(including nodes, edges, features, and classes for node/edge datasets and graphs, average nodes, average edges, and classes for graph datasets) of the real-world graph datasets used in this paper. We report the statistics of these real-world datasets in Table~\ref{table:grpah-statistics}. The descriptions of each of these datasets and their data splits are listed as follows:
\begin{itemize}[leftmargin=14pt]
    \item \textbf{Cora, CiteSeer, and PubMed} are academic citation networks originally introduced in~\cite{yang2016revisiting}, which are the most widely used benchmark datasets for semi-supervised node classification~\cite{yang2016revisiting}. In these networks, nodes represent papers and edges denote the citation of one paper by another. Node features are the bag-of-words representation for each node and the node label is the academic topic of a paper. We follow the public fixed split from~\cite{yang2016revisiting}. We use 20 samples per class for the training set, and 500 and 1000 samples in total for the validation and the testing set, respectively.
    \item \textbf{Chameleon and Squirrel} are two page-page graphs on specific topics in Wikipedia network~\cite{rozemberczki2021multi}. In these datasets, nodes represent the web pages and edges denote mutual links between pages. Node features are several informative nouns on Wikipedia pages. We follow the node labels generated by~\cite{pei2020geom}, where nodes are classified into five categories in terms of the number of the average monthly traffic on the web page. Following~\cite{pei2020geom}, we randomly split nodes of each class into 60\%, 20\%, and 20\% for the training, the validation, and the testing set.
    \item \textbf{Actor} is the actor co-occurrence induced subgraph of the film-director-actor-writer network~\cite{tang2009social}. In this network, nodes represent actors and the edge between two nodes denotes the co-occurrence on the same Wikipedia page. Node features are generated by some pre-defined keywords on Wikipedia pages. Following the node labels generated by~\cite{pei2020geom}, we classify the nodes into five categories in terms of words from the corresponding actor's Wikipedia. Following~\cite{pei2020geom}, we randomly split nodes of each class into 60\%, 20\%, and 20\% for the training, the validation, and the testing set.
    \item \textbf{Cornell, Texas, and Wisconsin} are webpage datasets of computer departments in universities, \ie Cornell, Texas, and Wisconsin. In these datasets, nodes represent web pages and edges denote the hyperlinks between them. Node features are the bag-of-words representation of corresponding web pages. We also follow the node labels generated by~\cite{pei2020geom}, where nodes are classified into five categories according to the identity of people. Following the method introduced in~\cite{pei2020geom}, we randomly split nodes of each class into 60\%, 20\%, and 20\% for the training, the validation, and the testing set.
    \item \textbf{OGBn-Arxiv} is a recently proposed large-scale dataset of paper citation networks~\cite{hu2020open}. Nodes represent arXiv papers and edges denote the citations between two papers. Node features are 128-dimensional feature vectors obtained by averaging the embeddings of words in the title and abstract and node labels are the primary categories of the arXiv papers. We use the public data split based on the publication dates of papers.
    \item \textbf{DD, NCI1, and PROTEINS} are chemical compound datasets introduced in~\cite{Morris+2020}. The nodes represent secondary structure elements~(SSEs) and edges between two nodes denote the neighborhood relationship in the amino-acid sequence or 3D space. We use a one-hot embedding vector to denote the features of different nodes. Node labels are categorized into two classes according to their chemical property. Following~\cite{errica2019fair}, we randomly split nodes of each class into 80\%, 10\%, and 10\% for the training, the validation, and the testing set.
    \item \textbf{IMDB-BINARY, REDDIT-BINARY} are social networks, representing movie collaboration and the online discussion forum, respectively. Nodes represent actors/actresses and users, respectively. Edges between two nodes denote they appear in the same movie in IMDB-BINARY and one user responds to another's comment in REDDIT-BINARY. We use a one-hot embedding vector to denote the features of different nodes. Node labels are categorized into two classes according to their community or subreddit. Following~\cite{errica2019fair}, we randomly split nodes of each class into 80\%, 10\%, and 10\% for the training, the validation, and the testing set.
\end{itemize}
