# Supplementary material for: AKE-GNN: Effective Graph Learning with Adaptive Knowledge Exchange
Source: arXiv:2106.05455 source file (2023-10-04)
Supplement: Supplementary file 3 [file AppendixE-experiments.tex]

\section{Experimental Setup}
\label{sec:appendix-experiments}
For reproducibility, we provide our experimental environment and all websites of the baseline GNN models and datasets. 
% Our codes and data are publicly available~\footnote{\url{https://tinyurl.com/AKE-GNN}}.
%, and implementation details. 
% The implementation details include the experimental settings, detailed hyper-parameters in their original papers that we follow, and the configurations of graph augmentation methods.

\subsection{Experiments Settings}
All experiments are conducted with the following settings:
\begin{itemize}[leftmargin=14pt]
    \item Operating system: Ubuntu Linux 16.04.7 LTS
    \item CPU: Intel(R) Xeon(R) Silver 4210 CPU @ 2.20GHz
    \item GPU: NVIDIA GP102GL [Tesla P40]
    \item Software versions: Python 3.7; Pytorch 1.7.0; Numpy 1.16.2; SciPy 1.2.1; Pandas 1.0.5; scikit-learn 0.23.1; PyTorch-geometric 1.6.3; Open Graph Benchmark 1.3.1
\end{itemize}

\subsection{Baseline GNNs and Datasets}
\label{sec:appendix-experiments}
We follow the experimental settings in their original paper. Table~\ref{table:gnn-url} summarizes URLs and commit numbers of baseline codes. Datasets used in this paper can be found in the following URLs, as shown in Table~\ref{table:dataset-url}. 

\begin{table}[h]
\centering
\small
\caption{Baseline GNNs.}
\label{table:gnn-url}
\scalebox{0.72}{
\begin{tabular}{lccc}
\toprule
                                      & Methods    & URL                                                                  & Commit  \\ \midrule
                                      & GCN        & \url{https://github.com/rusty1s/pytorch\_geometric} & db3bdc2 \\
                                      & GAT        & \url{https://github.com/rusty1s/pytorch\_geometric} & db3bdc2 \\
\multirow{5}{*}{Node classification}  & APPNP      & \url{https://github.com/benedekrozemberczki/APPNP}  & fce0d76 \\
                                      & JKNET-CAT  & \url{https://github.com/rusty1s/pytorch\_geometric} & db3bdc2 \\
                                      & JKNET-MAX  & \url{https://github.com/rusty1s/pytorch\_geometric} & db3bdc2 \\
                                      & GCNII      & \url{https://github.com/chennnM/GCNII}              & ca91f56 \\
                                      & GRAND      & \url{https://github.com/THUDM/GRAND}                & ba164c6 \\ \midrule
Edge prediction                       & GCN-EDGE   & \url{https://github.com/rusty1s/pytorch\_geometric} & e6b8d6  \\ \midrule
\multirow{2}{*}{Graph classification} & GCN-GRAPH  & \url{https://github.com/diningphil/gnn-comparison}  & 0e0e9b1 \\
                                      & GIN        & \url{https://github.com/rusty1s/pytorch\_geometric} & db3bdc2 \\ \midrule
\multirow{3}{*}{OGBn-Arxiv}           & GCN-RES-v2 & \url{https://github.com/ytchx1999/GCN\_res-CS-v2}   & a3e7d1f \\
                                      & GCN-DGL    & \url{https://github.com/Espylapiza/dgl}             & 5feada0 \\
                                      & GraphSAGE  & \url{https://github.com/snap-stanford/ogb}          & be38132 \\ \bottomrule
\end{tabular}
}
\end{table}

\begin{table}[h]
\caption{Datesets.}
\centering
\small
\label{table:dataset-url}
\scalebox{0.82}{
\begin{tabular}{cc}
\toprule
Datasets                   & URL                                                                                                \\ \midrule
Cora, CiteSeer, PubMed     & \url{https://github.com/rusty1s/pytorch\_geometric}   \\
Chameleon, Squirrel        & \url{https://github.com/graphdml-uiuc-jlu/geom-gcn}                                \\
Actor                      & \url{https://github.com/graphdml-uiuc-jlu/geom-gcn}                                \\
Cornell, Texas, Wisconsin  & \url{https://github.com/graphdml-uiuc-jlu/geom-gcn}                                \\
DD, NCI1, PROTEINS         & \url{https://github.com/rusty1s/pytorch\_geometric} \\
IMDB-BINARY, REDDIT-BINARY & \url{https://github.com/rusty1s/pytorch\_geometric} \\
OGBn-Arxiv                 & \url{https://github.com/snap-stanford/ogb}                  \\ \bottomrule
\end{tabular}
}
\end{table}
